# Supplementary material for: OVANet: One-vs-All Network for Universal Domain Adaptation
Source: arXiv:2104.03344 source file (2021-08-24)
Supplement: Supplementary file 3 [file anomaly_supple.tex]

\begin{table*}[ht]
\begin{center}
 %\addtolength{\tabcolsep}{-3pt}

\begin{tabular}{@{}c|c|cccc@{}}

\toprule[1.5pt]
$\mathcal{D}_{\text{in}}$ & $\mathcal{D}_{\text{out}}$  &Acc &UNK&H-Score / Best &Overall Acc / Best\\ \midrule
%\parbox[t]{2mm}{\multirow{4}{*}{\rotatebox[origin=c]{90}{\small CIFAR-10}}} 
\multirow{2}{*}{CIFAR-10} & CIFAR-100      &91.9 &67.1&77.5 / 85.3&79.5 / 85.5\\
 & SVHN            &91.9 &84.6&88.1 / 91.3&86.7 / 93.8 \\
\midrule
% \parbox[t]{2mm}{\multirow{4}{*}{\rotatebox[origin=c]{90}{\small CIFAR-100 80}}}
\multirow{3}{*}{CIFAR-100-80} & CIFAR-100-20       & 94.8 &63.1& 64.3 /  64.7 & 64.3 / 65.4\\
 & CIFAR-10        &94.8 & 69.0	& 67.2 / 67.3& 67.3 / 68.0\\
 & SVHN            & 94.8 & 74.5&69.7 / 69.8	& 72.0 / 80.9\\
 \bottomrule[1.5pt]
\end{tabular}
\caption{\textbf{Results in open-set recognition.} Acc shows the accuracy to accept the in-lier samples as known, UNK denotes the accuracy to reject the out-lier dataset as unknown. H-score considers the trade-off between Acc and UNK. \ours performs comparable well to \textit{Best} scores, which indicate that the decided threshold is close to the optimal one. }
\label{tab:anomay_csi}

\end{center}
\end{table*}
